# Supplementary material for: BANF: Band-limited Neural Fields for Levels of Detail Reconstruction
Source: arXiv:2404.13024 source file (2024-07-11)
Supplement: Supplementary file 1 [file 3D_color_supp_old.tex]

\begin{table*}[!tb]
\begin{tabular}{ccc|cc}
         & iNGP-64 & BANF-64 & iNGP-128 & BANF-128 \\ \hline
Chair    &    26.27     &         &          &          \\
Drums    &    21.85     &         &          &          \\
Ficus    &    24.06     &         &          &          \\
Hotdog   &    28.33     &         &          &          \\
Lego     &         &         &          &          \\
Material &         &         &          &          \\
Mic      &         &         &          &          \\
Ship     &         &         &          &          \\ \hline
Average  &         &         &          &         
\end{tabular}
\label{fig:3d-color}
\end{table*}
